# Supplementary material for: Natural Boundary Conditions for Smoothing in Geometry Processing
Source: arXiv:1707.04348 source file (2017-07-13)
Supplement: Supplementary file 1 [file old_appendix.tex]

% !TEX root = hessian.tex

\appendix
 
%\section{Green's indentities}
%We require \emph{Green's identities} for relating the biharmonic and Hessian
%energies, We repeat these identities here for keeping the exposition
%self-contained and since we require some non-standard equalities. The standard
%Green's identity is
%
%%bilinear integrals of $u$ and some other
%%function $v$ on the interior to integrals along the boundary:
%%

%\section{Dirichlet \& Neumann boundary conditions}
%\label{sec:hessianbdryderivation}
%%
%Dirichlet and Neumann boundary conditions yield the equivalence between
%%
%biharmonic and Hessian energy. Indeed, fixing Dirichlet ($u=f$) and Neumann
%($\partial_\n u = \dn{u}=g$) conditions, the boundary term satisfies
%\begin{align*}
%\int_{\partial\Omega} \nabla u^T (\H_u-\Delta u \I) \n \ds
%&= \int_{\partial\Omega} u_1(-u_{22} \n_1 + u_{12} \n_2) \ds\\ 
%&\quad +   \int_{\partial\Omega}  u_2(u_{12} \n_1 - u_{11} \n_2)  \ds \ .
%\end{align*}
%The first integral on the right can be rewritten as 
%\begin{align*}
%%\int_{\partial\Omega} u_1(-u_{22} \n_1 + u_{12} \n_2) \ds 
% \int_{\partial\Omega} u_1(-\partial_2 u_2 \n_1 + \partial_1 u_2 \n_2) \ds 
%=  -\int_{\partial\Omega} u_1 \partial_\t u_2  \ds \ ,
%\end{align*}
%where $\partial_\t$ denotes the tangential derivative along $\partial\Omega$. The terms of the product in the last integrand can be rewritten as
%\begin{align*}
%u_1 &= (\t \partial_\t u   + \n \partial_n u )  \cdot \e_1 =  (\t \partial_\t f  + \n g )  \cdot \e_1 \quad\text{and}\\
%\partial_\t u_2   &= \partial_\t ((\t \partial_\t u   + \n \partial_n u ) \cdot \e_2) = \partial_\t ((\t \partial_\t f   + \n g ) \cdot \e_2) \ ,
%\end{align*}
%which involves $f$ and $g$ but not $u$. Similar considerations hold for $u_2(u_{12} \n_1 - u_{11} \n_2)$. Consequently, the boundary term only depends on $f$ and $g$, but not on $u$.

%\section{Boundary term is constant for fixed Dirichlet and fixed Neumann}
%
%\alec{The formatting needs to be cleaned up to fit in two columns}
%
%Assume $\defon{u = f}{∂Ω}$ and $\defon{\dn{u} = g}{∂Ω}$:
%\begin{align}
%∮\limits_{∂Ω} \gT{u} \left(\H_u - ∆u\I\right) \n \ds, \\
%∮\limits_{∂Ω} \gT{u} \H_u \n - \gT{u} ∆u \n \ds, \\
%∮\limits_{∂Ω} \gT{u} \H_u \n - ∆u g \ds, \\
%\end{align}
%
%Assuming $f$ is tangentially differentiable then $\defon{\dt{u} = \dt{f}}{∂Ω}$.
%Let $\dt{f} = z$ then $∇u = z \t + g \n$. Consider the first term:
%
%\begin{align}
%\gT{u} \H_u \n &= \left(z \t + g \n\right)^\transpose \H_u \n \\
%               &= z \t^\transpose \H_u \n  + g \n^\transpose \H_u \n
%\end{align}
%\alec{seems like I want to show that $g \n^\transpose \H_u \n =  ∆u g$ and that
%$z \t^\transpose \H_u \n = \text{constant}$, but I'm not seeing it...}
%
% ∇u’ *(H_u-∆u I) n = gradu'*n * laplace u + gradu' * Hu * n = g laplace u + ut *
% Hu * n
% 
% [3:19]  
% where ut is the tangential derivative of u at the bdry
% 
% [3:20]  
% t' Hu n = (utn)^2, where utn is the derivetive of u in tangential and then
% normal direction
% 
% [3:21]  
% It follows that the whole thing is  g laplace u + u (gn)^2
% 
% [3:21]  
% sorr the last line was wrong
% 
% [3:22]  
% g laplace u + ut (gt)^2
% 
% [3:22]  
% that is the whole thing
% 
% [3:23]  
% ut should be fixed if the Dirichlet argument is correct
% 
% eitangrinspun [3:24 PM] 
% Is Max officially away today for the lord’s day?
% 
% alecjacobson [3:26 PM] 
% oded is your derivation complete? I think there’s a missing minus sign:∇u’
% *(H_u-∆u I) n = - gradu'*n * laplace u + gradu' * Hu * n = - g laplace u + ut *
% Hu * n
% 
% odedstein [3:26 PgM

\section{$L^1$ minimization}
\label{app:qp}

In the smooth setting, the \(L^1\) norm of the Laplacian
is:
%
\begin{equation}\label{eq:l1smoothlaplacian}
%
 D_L(u) = \int_\Omega \left| \Delta u(x) \right|\dx
%
\end{equation}

This can be minimized for discretized functions in the following way: if
\(D_L(u) < \varepsilon\), then it holds: 
%
\begin{equation}\begin{split}
%
 \sum_{i,j} s_x s_y | \Delta u_{i,j} | &< \varepsilon \\ 
%
 | \Delta u_{i,j} | &< y_{i,j} \; \forall i,j  \quad \sum_{i,j} s_x s_y y_{i,j} = \varepsilon  \\
%
 -y_{i,j} < \Delta u_{i,j} &< y_{i,j} \; \forall i,j  \quad \sum_{i,j} s_x s_y y_{i,j} = \varepsilon 
%
\end{split}\end{equation}
%
for some positive function \(y\).

This gives the following linear programming problem:
%
\begin{equation}\begin{split}
 \argmin_{\u,\y} &\; \mathbf{1}^T \M y \\
 \L\u &\geq -y \\
 \L\u &\leq y \\
 y &\geq 0
\end{split}\end{equation}
%
where \(\mathbf{1}\) is a vector of ones of appropriate length, with \(\tilde
\L\) instead of \(\L \) for the zero Neumann Laplacian. The linear programming
problem for the Hessian is derived analogously. It is:
%
\begin{equation}\begin{split}
 \argmin_{\u,\y} &\; \mathbf{1}^T \M_4 \y \\
 \H \u &\geq -\y \\
 \H \u &\leq \y \\
 \y &\geq 0
\end{split}\end{equation}

This can be combined with the (quadratic) fidelity energy to get a quadratic
programming problem for minimizing the \(L^1\) norm of Laplacian and Hessian.\\

%\input{point-constraints}

\section{Finite Differences}
\label{app:fd}

In order to discretize $E_{\H²}$ over a domain $Ω$ embedded in a $n_x×n_y$-node
grid, we define a sparse matrix $\H = \left[\H_{xx}^\transpose\
\H_{yy}^\transpose\ \sqrt{2}\H_{xy}^\transpose\right]^\transpose \in \R^{3m ×
n}$ so that each row of $\H_{xx}$ approximates the second derivative of the
unknown function at the corresponding interior grid node: $\H^i_{xx} \u \approx
∂²u(\x_i)/∂x²$ and analogously for rows in $\H_{yy}$ and $\H_{xy}$.

We use standard, second-order stencils for each term, i.e.,:
%
\begin{align}
\H_{xx}^i\u                  &= \frac{u_{i  ,j-1} -2 u_{i  ,j}+u_{i  ,j+1}}{h²}\\
\H_{yy}^i\u                  &= \frac{u_{i-1,j  } -2 u_{i  ,j}+u_{i+1,j  }}{h²} \\
\H_{xy}^i\u = \H_{yx}^i\u    &= \frac{u_{i-1,j-1} +u_{i-1,j+1}-u_{i+1,j-1}+u_{i+1,j+1}}{4h²}.
\end{align}

\section{Mixed Finite Elements}
\label{app:mfem}



%
Solving this problem by differentiating with respect to all degrees of freedom,
we have a system of linear equations in matrix form:
%
% ∫ (∇⋅V)⋅∇u dA
% ∫ Vij,j u,i dA
%
\begin{equation}
%
\left(\begin{array}{cc}
\MM 
  & \G^\transpose 
  \A
  % \left(\begin{array}{cc}
  % \A & 0 \\
  % 0  & \A
  % \end{array}\right)
  \D \\
\D^\transpose 
  \A
  %\left(\begin{array}{cc}
  %\A & 0 \\
  %0  & \A
  %\end{array}\right)
  \G & 0
\end{array}
\right)
\left(\begin{array}{cc}
\V_{xx} \\
\V_{xy} \\
\V_{yx} \\
\V_{yy} \\
\u      
\end{array}
\right)
= 0
%
\end{equation}
where $\MM ∈ \R^{4|i|×4|i|}$ repeats the mass matrix $\M(i,i)$ along the
diagonal, $\A∈\R^{2m×2m}$ is a diagonal matrix containing triangle areas, and
$\D ∈ \R^{2m×4|i|}$ computes the matrix divergence defined by:
%
\begin{equation}
\D = 
%
\left(\begin{array}{cccc}
%
\G(x,i) & \G(y,i) & 0       & 0 \\
      0 &       0 & \G(x,i) & \G(y,i)
\end{array}\right),
%
\end{equation}
where $\G ∈ \R^{2m × n}$ is the usual gradient operator and $\G(x,i)$ selects
the rows and columns corresponding to the $x$-components and interior vertices
respectively.
%
Finally, if we use lumped mass matrices we can condense this system and use it
to define a discretization of our original energy:
%
\begin{equation}
E_{\H^2}(u) ≈ \u^\transpose \G^\transpose \A \D \MM^{-1}
\D^\transpose \A \G \u.
\end{equation}

\section{Figure Graveyard}

\begin{figure}
 \centering
  \includegraphics[width=0.5\textwidth]{images/smoothing/pacman.pdf}
  \caption{Pacman, L2 smoothing \label{fig:pacman}. The Laplacian
  with zero Neumann boundary conditions bends the isolines
  heavily along the eye of the Pacman in order to fulfill the
  zero Neumann boundary condition. The Hessian continues the
  isolines across the eye as linearly as possible.}
 %\end{center}
\end{figure}

\begin{figure}
\includegraphics[width=\linewidth]{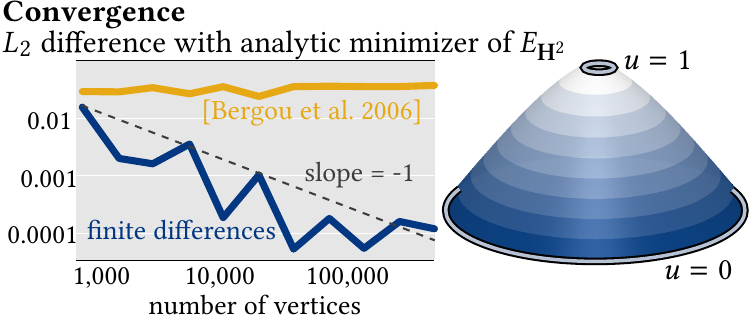}
\caption{Our discretizations converge to analytic solutions on an annular
domain. Fixing values at the outer and inner boundary, we consider the squared
Laplacian energy $E_{\Delta^2}$ with natural boundary conditions, with zero Neumann
boundary conditions $\dn{u}=0$, and the squared Hessian energy
$E_{\H^2}$ with natural boundary conditions.
\label{fig:annulus}}
\end{figure}

\begin{figure}
 \centering
  \includegraphics[width=\linewidth]{images/diamond-square.pdf}
  \caption{Our solution on an axis-aligned square matches our rotated solution
  on diamond under refinement. \label{fig:diamondsquare}}
 %\end{center}
\end{figure}

\begin{figure}
 \centering
  \includegraphics[width=\linewidth]{images/scattereddata/scattereddata.pdf}
  \caption{Scattered data interpolation over a country-shaped
    domain. The Laplacian energy subject to zero Neumann boundary
    conditions flattens the data at the boundary. Arrows \textsf{a}
    and \textsf{b} point to distortion of isolines due to the shape of
    the boundary. The Hessian energy over $\R^2$ ignores the geometry
    of the boundary completely and is sensitive to relative
    arrangement of data samples. Arrow \textsf{c} points to isolines
    that flow northwest along an open corridor; arrow \textsf{d}
    points to an information ``leak' from south to north across the
    boundary. The Hessian energy subject to its natural boundary
    conditions and data sample conditions alleviates these
    distortions, and extrapolates the data as linearly as
    possible (arrow $\textsf{e}$). \label{fig:scattereddata}}
 %\end{center}
\end{figure}

\begin{figure}
 \centering
  \includegraphics[width=0.5\textwidth]{images/checkerboard_test/checkerboards.pdf}
  \caption{Bending a straight checkerboard. Each red dot
  represents a group of 16 handles that are transformed together.
  For the noisy deformations, the handles are randomly moved in
  addition to the transformation. \label{fig:checkerboard}}
 %\end{center}
\end{figure}
\begin{figure*}
 \centering
  \includegraphics[width=\textwidth]{images/giraffe_test/giraffeplusweights.pdf}
  \caption{This shows a giraffe under ARAP deformation driven by
  LSD and Hessian subspaces respectively. Both methods perform
  similarly with a high number of extra handles, but the Hessian
  degrades gracefully as handles are removed while linear
  subspace design does not. \label{fig:giraffe}}
 %\end{center}
\end{figure*}
%
%\begin{figure}
% \centering
%  \includegraphics[width=0.5\textwidth]{images/greece.pdf}
%  \caption{Peak-shaped noisy data, L2-smoothed over a country-like domain. Laplacian with zero Neumann flattens the height field near the boundary, causing crease-like artifacts (amplified by the lighting). Hessian does not have this problem. \label{fig:greece}}
% %\end{center}
%\end{figure}

\begin{figure}
 \centering
  \includegraphics[width=0.5\textwidth]{images/l1-squares.pdf}
  \caption{
  \alec{It'd be nice to show a simple L2 vs L1 example like this, but this
  figure is very big and hard to see differences. Height field might be
  better.}
  The Manhattan distance function, \(L^1\)-denoised over a square
  domain. The Laplacian with zero Neumann boundary conditions introduces little
  bumps along the ridges where the piecewise linear functions meet, and it also
  bends the isolines to be normal to the boundary. The Hessian correctly
  reconstructs the piecewise linear function. \label{fig:squarel1}}
 %\end{center}
\end{figure}

\begin{figure}
 \centering
  \includegraphics[width=0.5\textwidth]{images/cheese_rigs/cheese_both.pdf}
  \caption{\alec{One reviewer complained about ``distortion''.} \alec{This
  figure has too much white space}. The cheeseman jumps in the top row, trips in the
  bottom, powered by Hessian weight functions.
  \label{fig:cheeseman}}
 %\end{center}
\end{figure}
